# Supplementary material for: Bayesian detection of unmodeled bursts of gravitational waves
Source: arXiv:0809.2809 source file (2009-06-04)
Supplement: Supplementary file 1 [file appendix.tex]

\section{better noise model}

The assumption that the interferometer noise is well-modeled by a multivariate normal distribution is convenient, but false.  The presence of `glitches' in the interferometer, where the noise statistics change dramatically, is well documented.  Current methods, including ours in the form proposed in the paper, are easily fooled by these bursts of excess power, simply because the analyses assume that the only way that extra power can be introduced to the interferometer is by a gravitational wave.  The gravitational wave hypothesis $H_\mathrm{signal}$ will do a very poor job of explaining temporally coincident incoherent bursts of noise power in the interferometer, but the noise hypothesis $H_\mathrm{signal}$ in its simple form does even worse; the gravitational wave explanation is thus preferred.

We can generalize the noise hypothesis to cope with glitches by creating a model for glitches and adding that hypothesis to the set under consideration.  Like gravitational waves, glitches are infrequent, have poorly known waveforms, and poorly known power.  Unlike gravitational waves, they will not be correlated between instruments.

%The Gursel-Tinto method is not robust against interferometer glitches (nor does it claim to be; real interferometer data doesn't follow the normal distribution assumed in the derivation of the method.)  This is a problem in naive attempts to use the Gursel-Tinto algorithm as a search.  Excess energy of any almost any kind will be interpreted as a evidence of a gravitational wave.  An \emph{ad hoc} addition to the method was propsed in \cite{us}.  A better way forward is to use a noise model that more accurately reflects the 'bursty' or 'glitchy' nature of the data, by replacing the normal noise distribution with a long-tailed distribution.  An immediate problem is that the marginalization integral does not in general have a closed form solution for such distributions.  If we model the long-tailed distribution using two normal distributions the marginalization integral remains tractable.

One first attempt at such a hypothesis is to propose that an interferometer is either `quiet' with some probability $p(H_\mathrm{quiet}|H_\mathrm{noise})$ and has a unit normal noise distribution, or is `glitching' with probability $p(H_\mathrm{glitch}|H_\mathrm{noise})$ and has an increased standard deviation $\sigma_g$

\begin{equation}
P(\mathbf{x}|H_\mathrm{noise})
=
\prod_{i=1}^{N}\left[p(H_\mathrm{quiet}|H_\mathrm{noise})
(2\pi)^{-n/2}
\exp(-\frac{1}{2}\sum_{j=1}^n x_{ij}^2)
+p(H_\mathrm{glitch}|H_\mathrm{noise})
(2\pi)^{-n/2}\sigma_g^{-n}
\exp(-\frac{1}{2\sigma_g^2}\sum_{j=1}^n x_{ij}^2)
\right]\label{eq:glitchy}
\end{equation}

If there is excess energy in only one detector, the new noise hypothesis will readily explain it.  If there is excess energy in three detectors, the noise hypothesis must invoke three coincident glitches and is penalized by $p(H_\mathrm{glitch}|H_\mathrm{noise})^3$ reflecting our belief that triple-coincidence glitches are rare, and the prediction that the glitches are incoherent thinly spreads the hypothesis over a higher-dimensional space than that of the signal hypothesis, which is concentrated around $\mathrm{span}\,\mathbf{F}$. These factors make it possible for the gravitational wave hypothesis to be preferred for some data.
